# Supplementary material for: SoulX-LiveAct: Towards Hour-Scale Real-Time Human Animation with Neighbor Forcing and ConvKV Memory
Source: arXiv:2603.11746 source file (2026-03-18)
Supplement: Supplementary file 1 [file Appendix.tex]

\section{Appendix}
